# Supplementary material for: Assessing treatment effect heterogeneity in the presence of missing effect modifier data in cluster-randomized trials
Source: arXiv:2209.01297 source file (2023-12-01)
Supplement: Supplementary file 1 [file Supplementary_Information_for_HTE_paper_revision_final.pdf]

**Supplementary Information for "Assessing treatment effect heterogeneity in the presence of missing effect modifier data in cluster-randomized trials"**

Bryan S. Blette, Scott D. Halpern, Fan Li, Michael O. Harhay

Table of Contents:

Page 2....................Web Figure 1
Page 3....................Web Figure 2
Page 4....................Web Figure 3
Page 5....................Web Figure 4
Page 6....................Web Figure 5
Page 7....................Web Figure 6
Page 8....................Web Figure 7
Page 9....................Web Table 1
Page 10....................Web Table 2
Page 11....................Web Table 3
Page 12....................Web Table 4

Web Figure 1: Simulation results for the ATE estimand in Scenario 1 of the simulation study when $\gamma_3$ = 0 (such that ATE = 1).

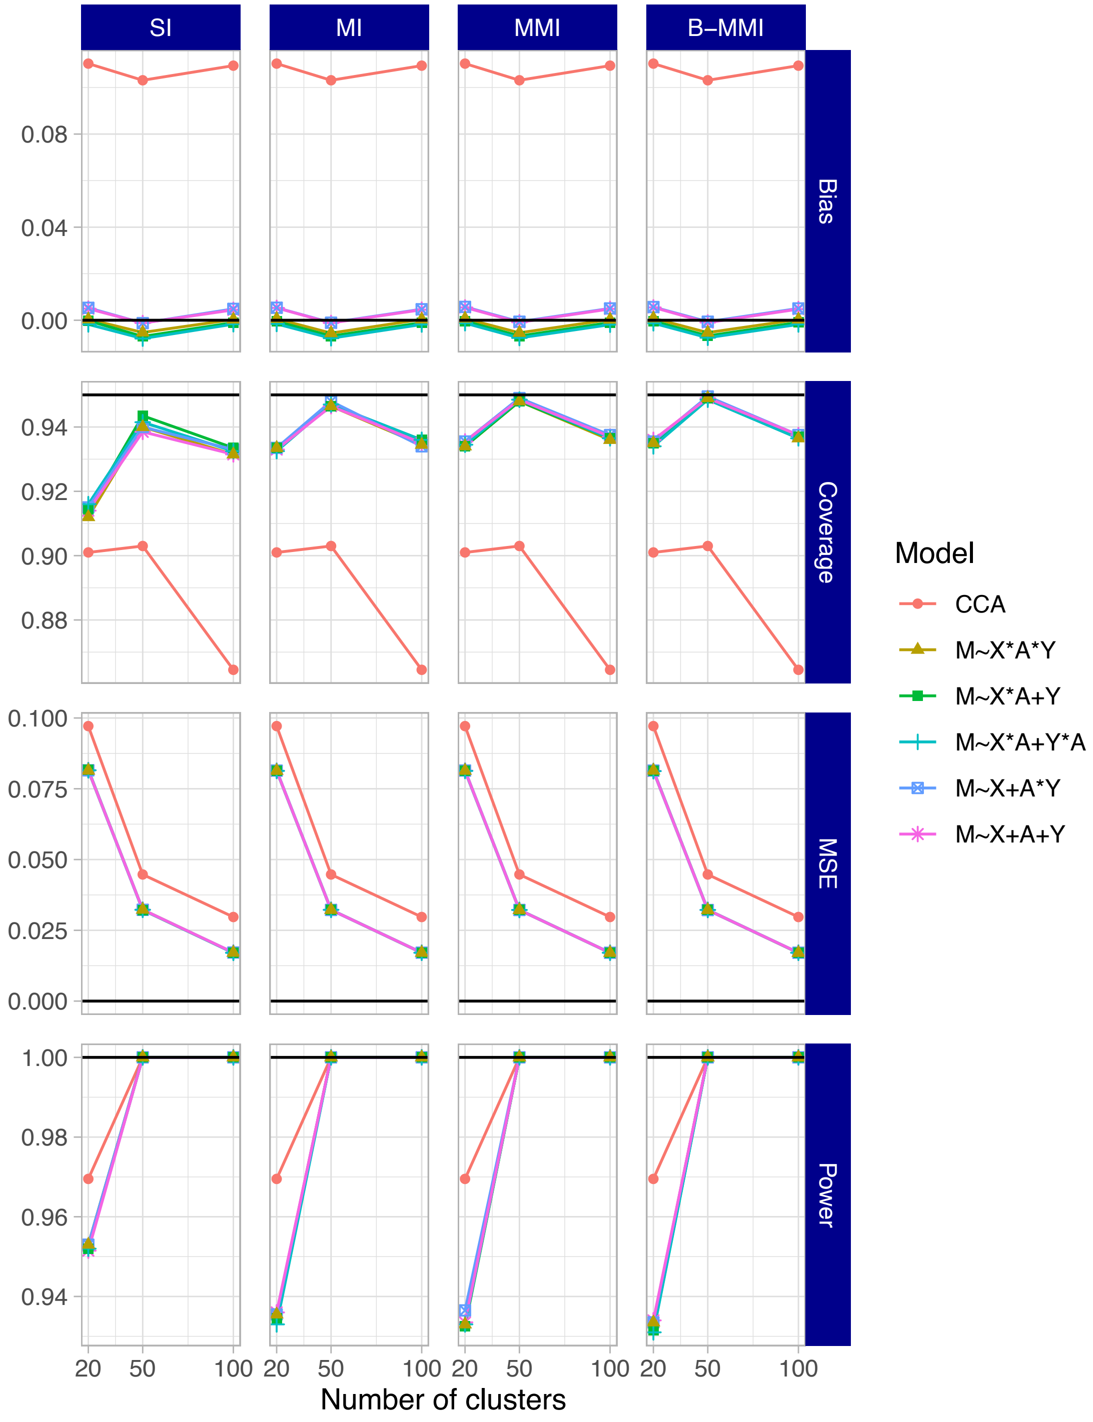

Web Figure 2: Simulation results for the HTE estimand (interaction effect estimand $\gamma_3$) in Scenario 1 of the simulation study when $\gamma_3$ = -{1 + exp(-0.5)}.

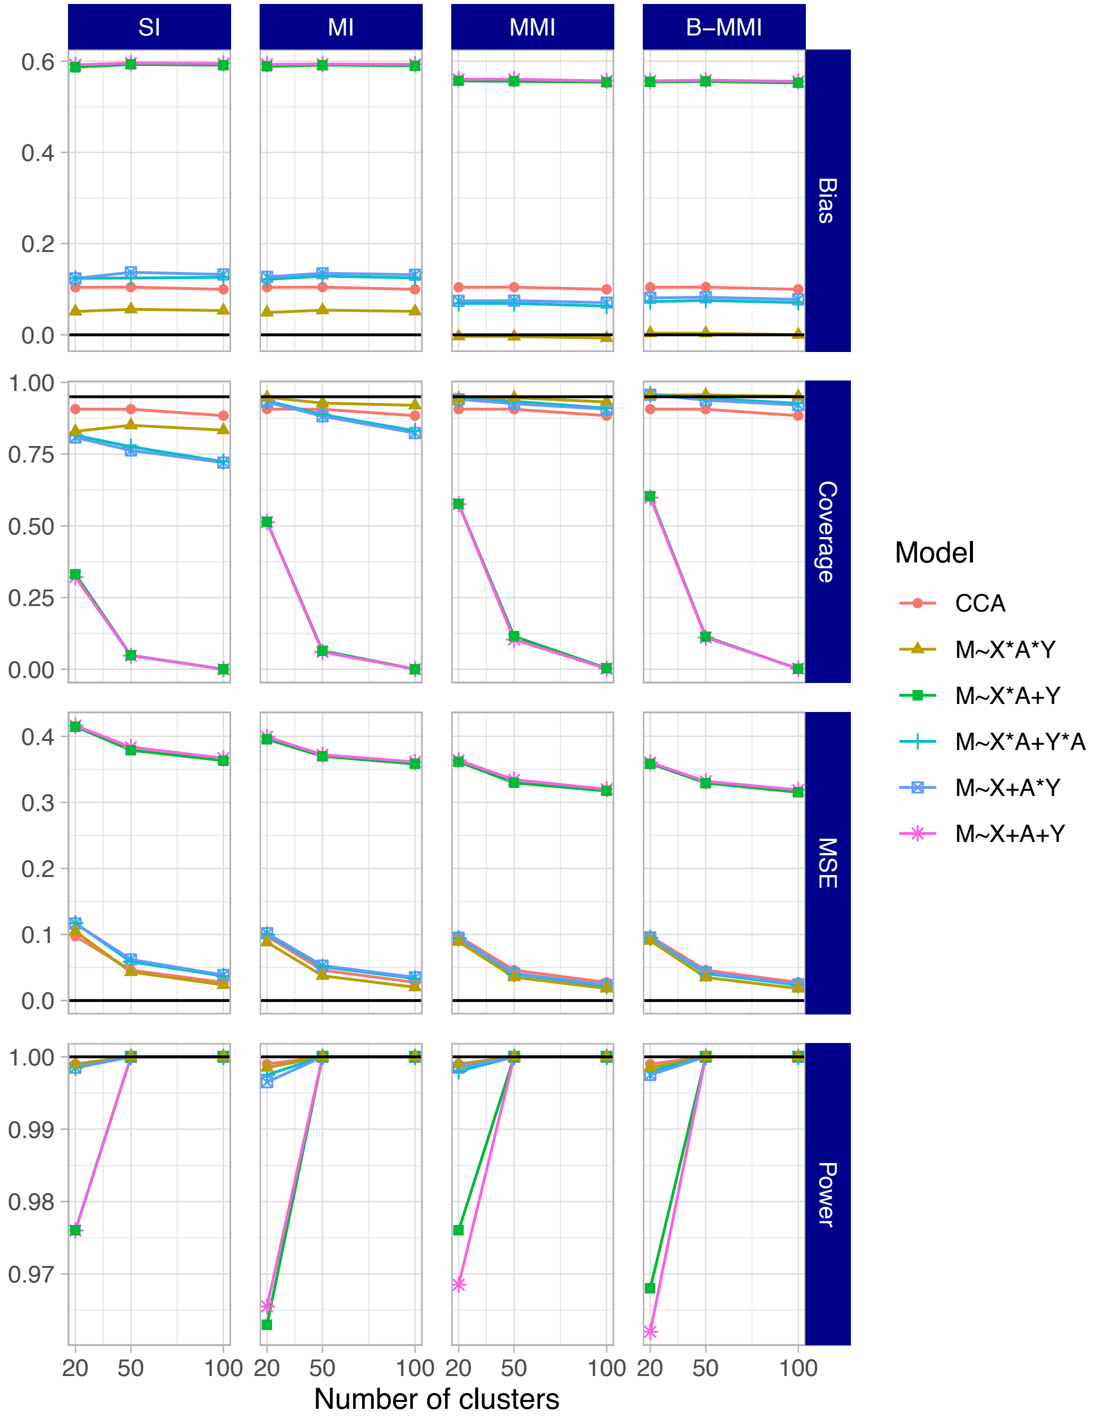

Web Figure 3: Simulation results for the ATE estimand in Scenario 1 of the simulation study when $\gamma_3$ = -{1 + exp(-0.5)} (such that ATE = 0).

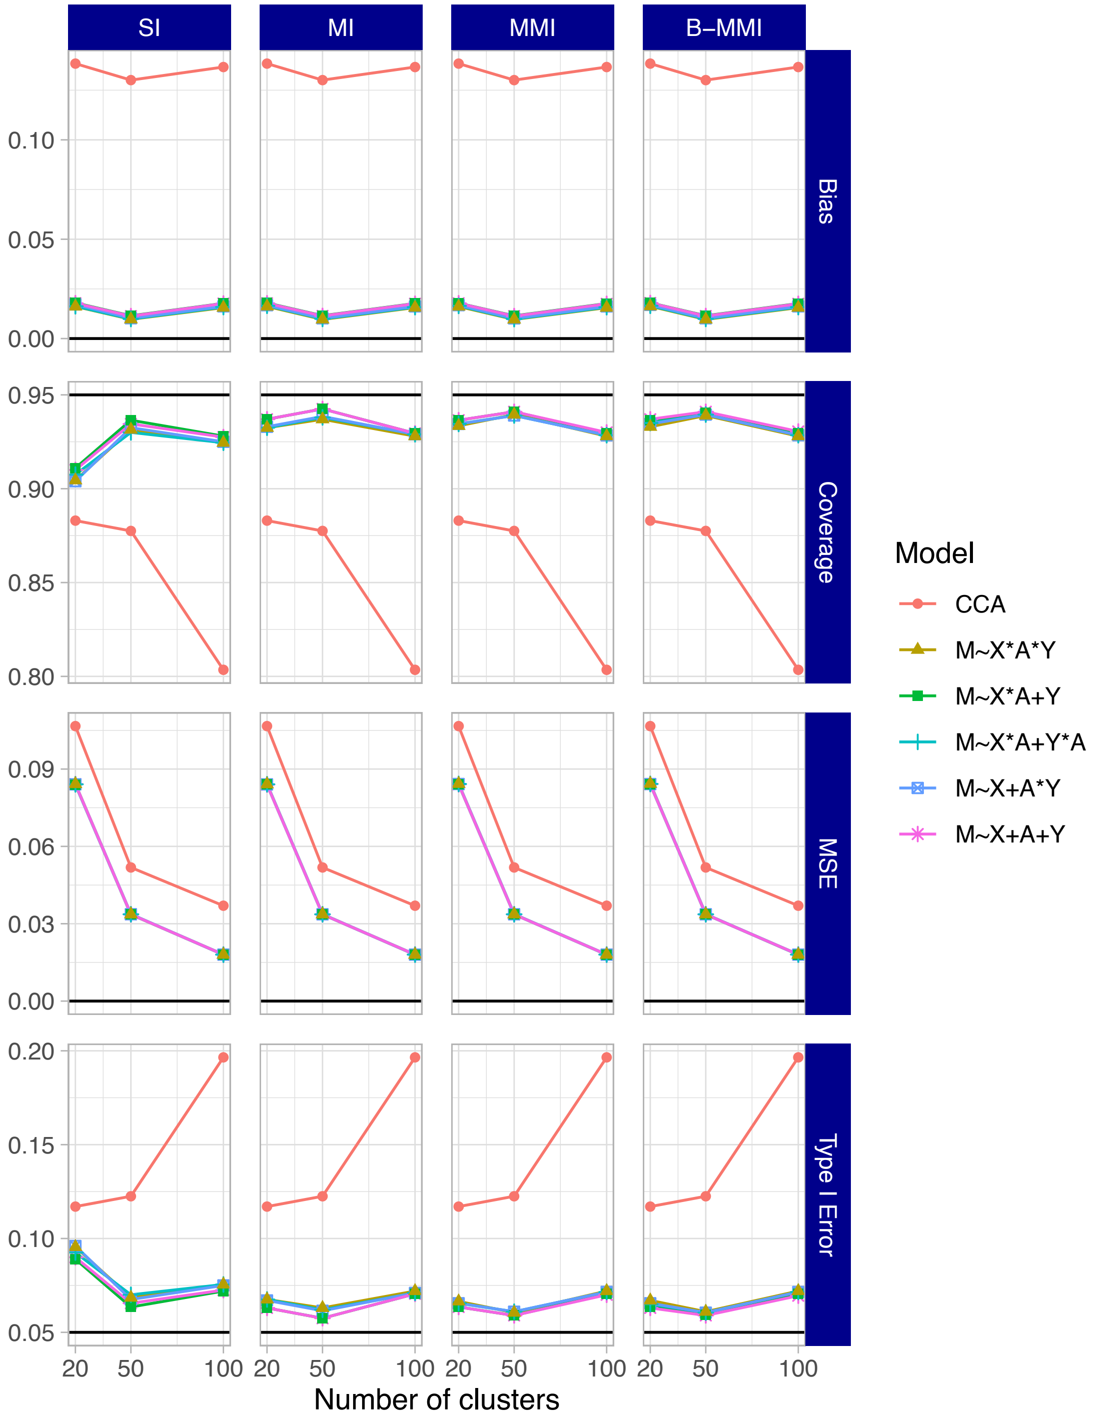

Web Figure 4: Simulation results for the ATE estimand in Scenario 2 of the simulation study when $\gamma_3$ = 0 (such that ATE = 1).

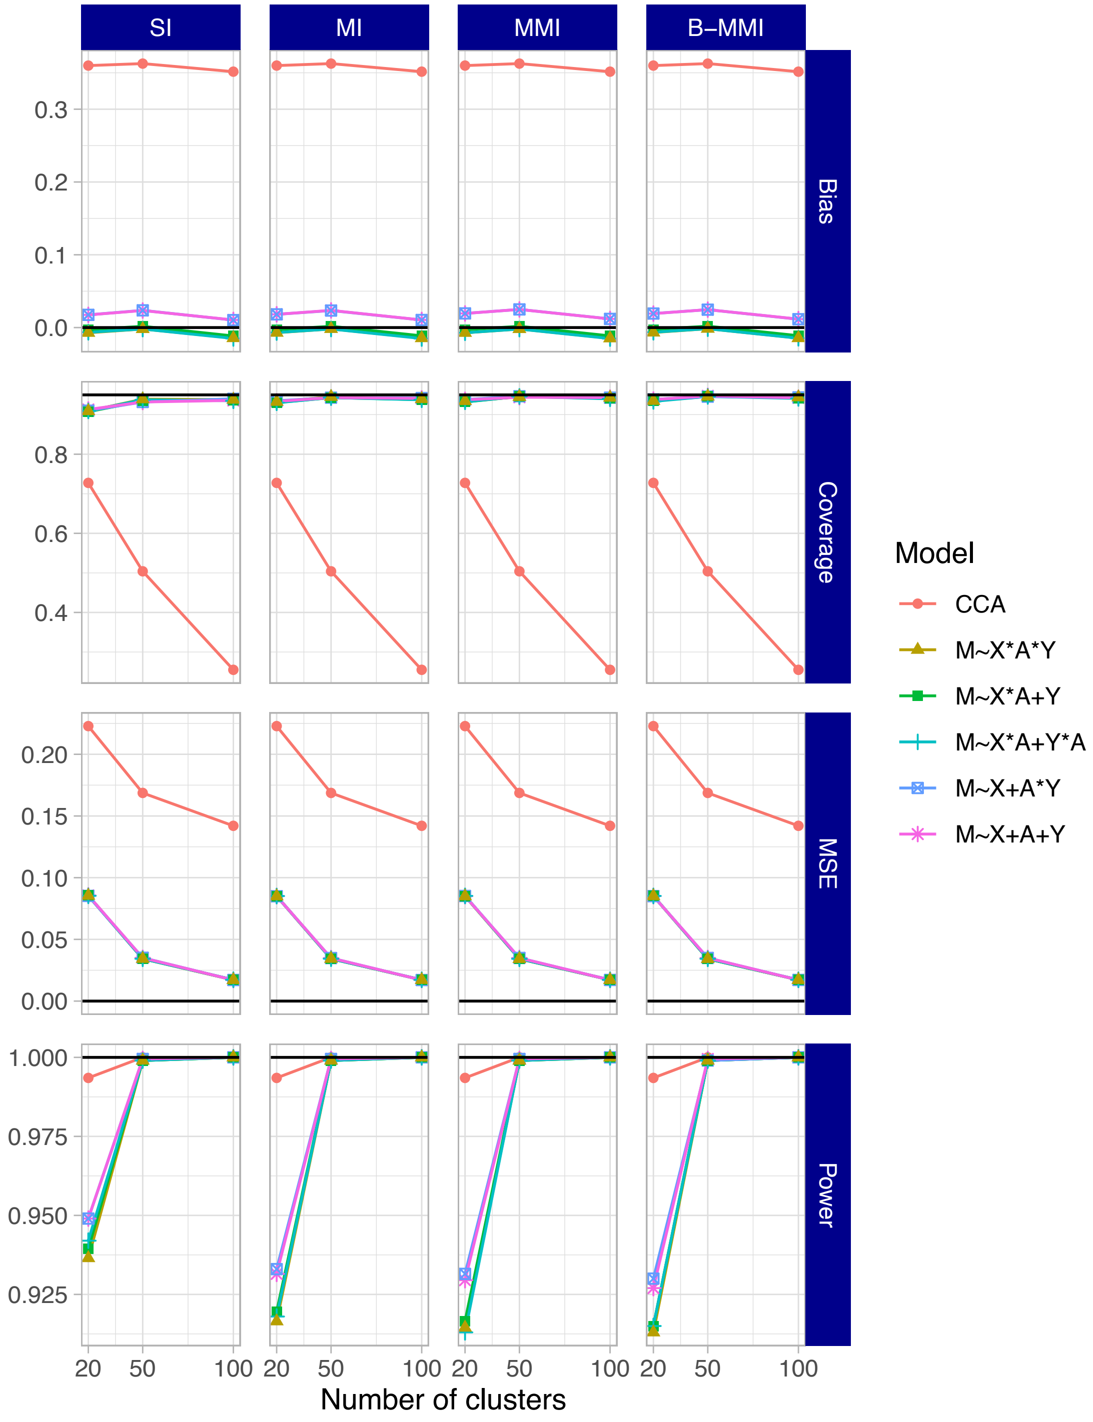

Web Figure 5: Simulation results for the HTE estimand (interaction effect estimand $\gamma_3$) in Scenario 2 of the simulation study when $\gamma_3 = -\{1 + \exp(-0.5)\}$.

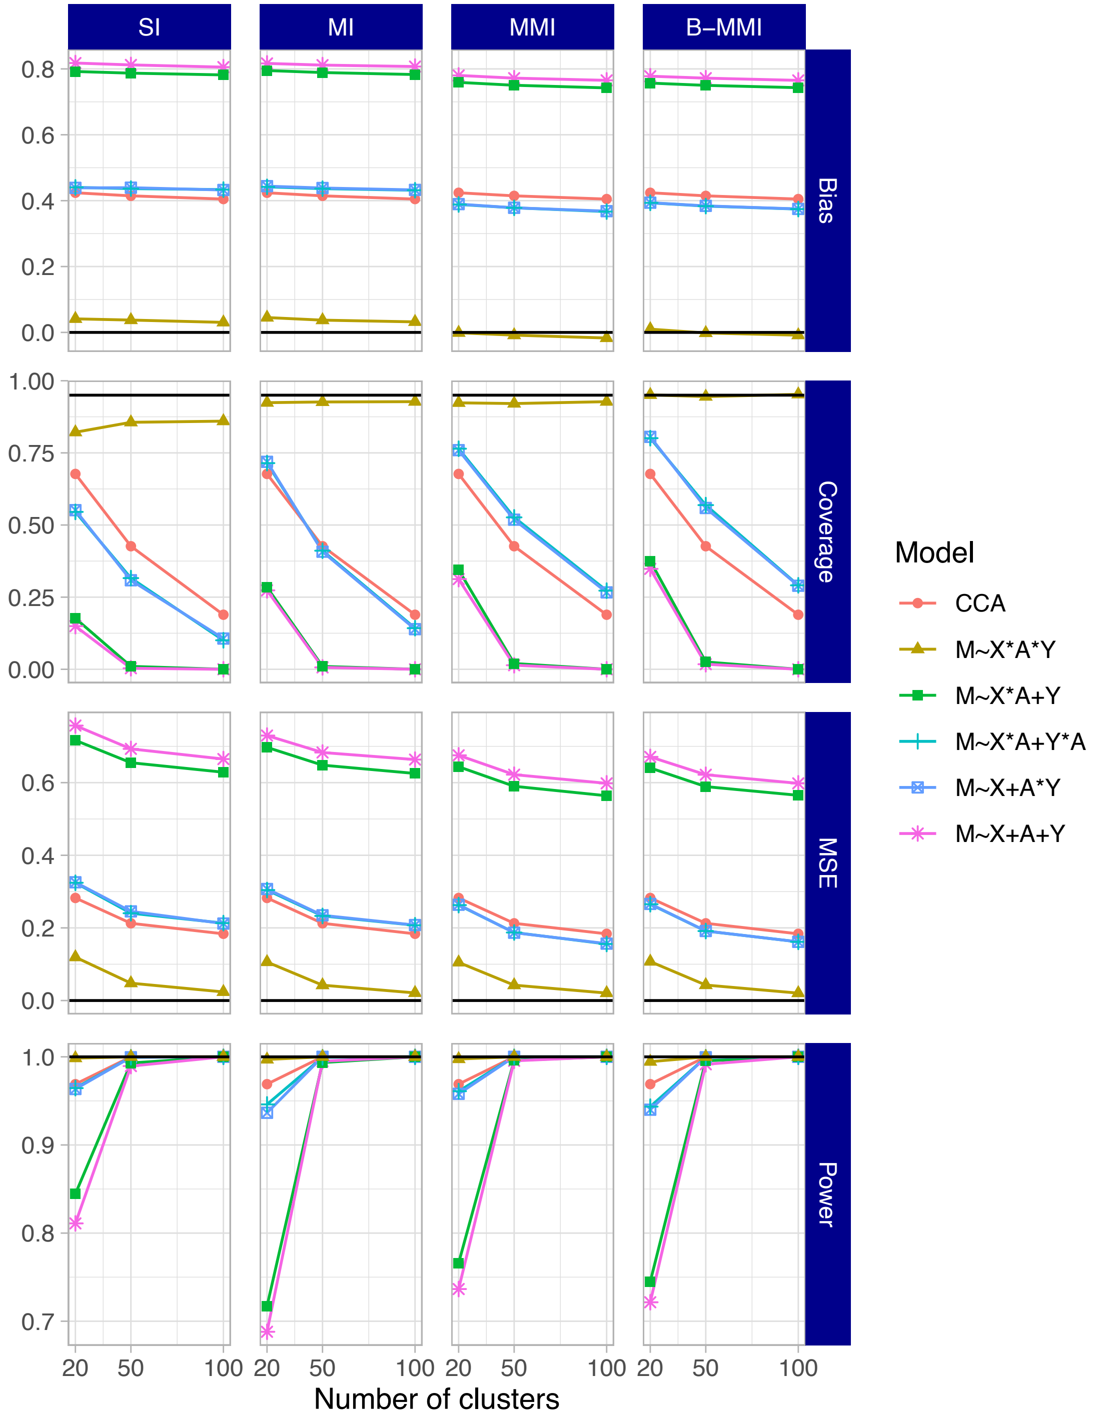

Web Figure 6: Simulation results for the ATE estimand in Scenario 2 of the simulation study when $\gamma_3$ = -{1 + exp(-0.5)} (such that ATE = 0).

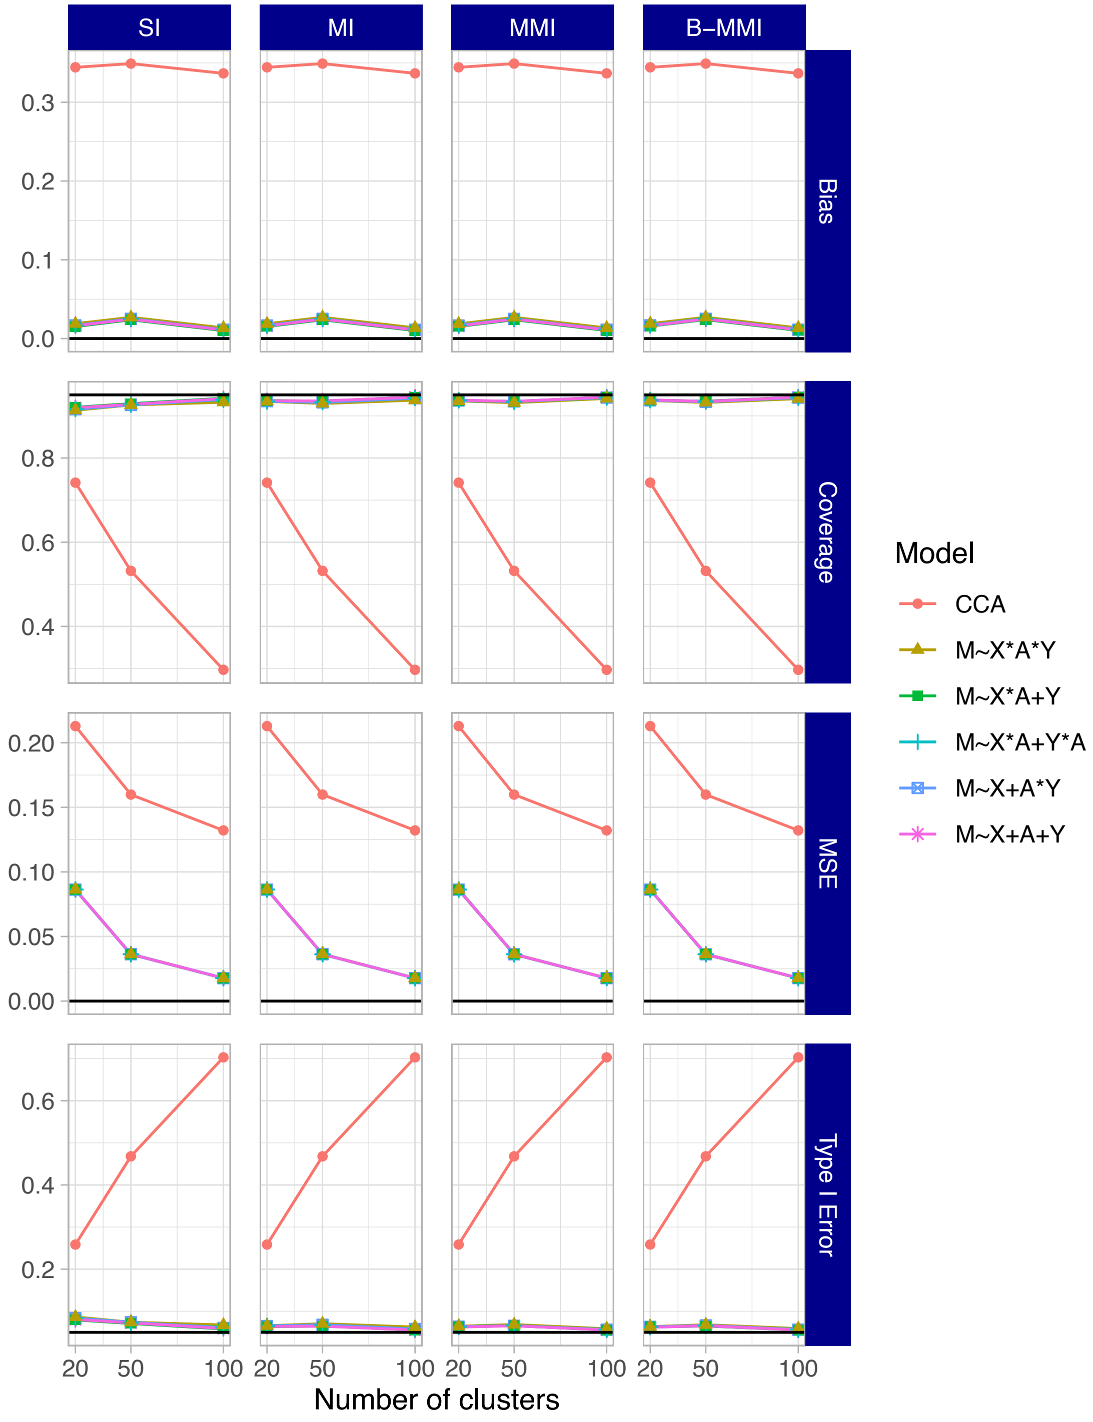

Web Figure 7: Results for the Work, Family, and Health Study data application. The top row shows box plots of point estimates for each method across 500 replications of the simulation procedure for the ATE estimand. The bottom row shows parallel results for the HTE estimand. The point estimate and 95% confidence interval estimated using the complete data are given on the left of each panel as a reference.

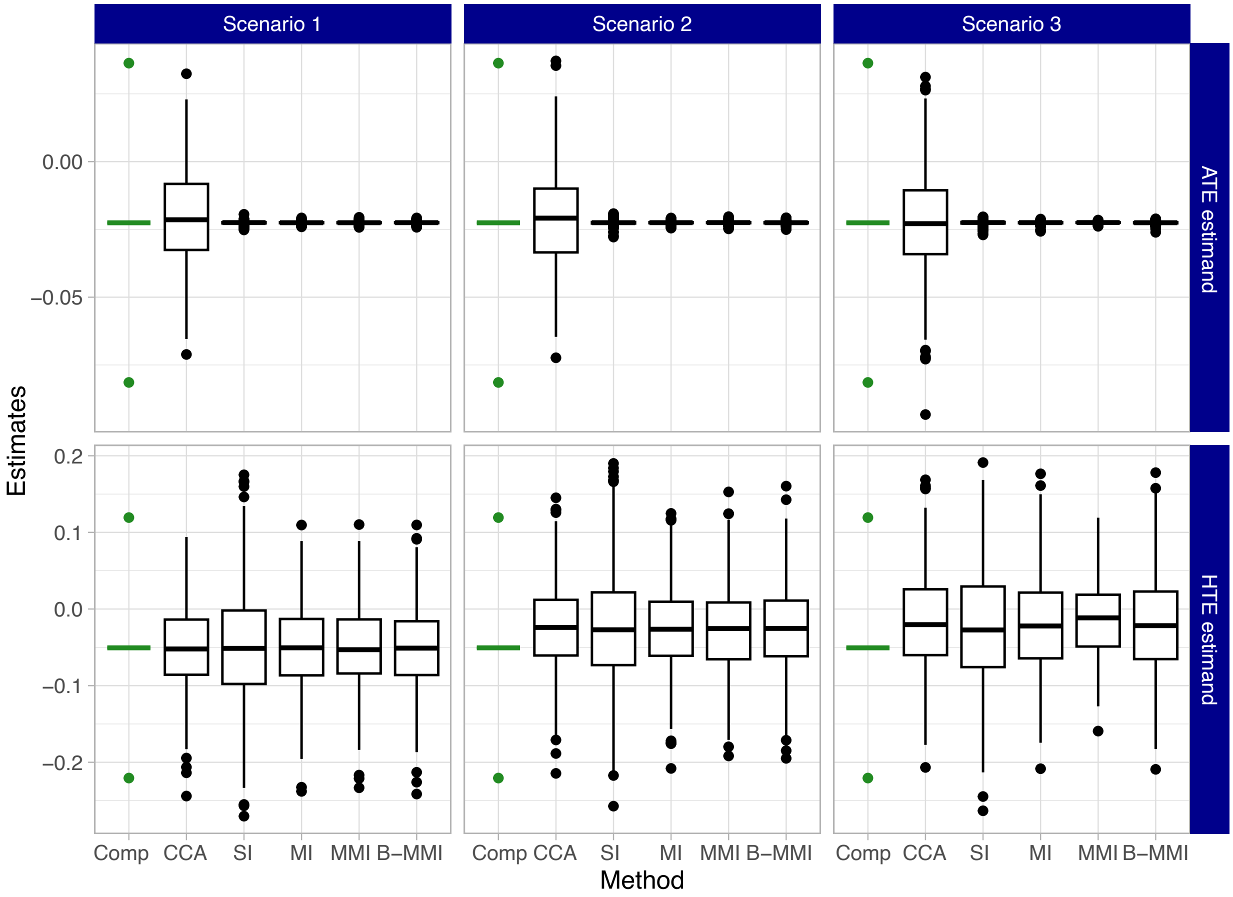

Web Table 1: Proportion of confidence intervals narrower than the complete data confidence interval for each method for the ATE estimand

| **Scenario** | **CCA** | **SI** | **MI** | **MMI** | **B-MMI** |
|---|---:|---:|---:|---:|---:|
| Scenario 1 | 0.150 | 0.486 | 0 | 0 | 0 |
| Scenario 2 | 0.162 | 0.358 | 0 | 0 | 0 |
| Scenario 3 | 0.142 | 0.410 | 0 | 0 | 0 |

Web Table 2: Proportion of confidence intervals narrower than the complete data confidence interval for each method for the HTE estimand (interaction effect estimand $\gamma_3$)

| Scenario | CCA | SI | MI | MMI | B-MMI |
|---|---|---|---|---|---|
| Scenario 1 | 0.138 | 0.336 | 0.000 | 0.002 | 0.002 |
| Scenario 2 | 0.106 | 0.252 | 0.002 | 0.000 | 0.000 |
| Scenario 3 | 0.090 | 0.222 | 0.000 | 0.004 | 0.000 |

Web Table 3: Proportion of confidence intervals which covered the complete data confidence interval for each method for the ATE estimand

| **Scenario** | **CCA** | **SI** | **MI** | **MMI** | **B-MMI** |
|---|---|---|---|---|---|
| Scenario 1 | 0.342 | 0.290 | 1 | 1.000 | 1 |
| Scenario 2 | 0.322 | 0.366 | 1 | 0.998 | 1 |
| Scenario 3 | 0.382 | 0.344 | 1 | 1.000 | 1 |

Web Table 4: Proportion of confidence intervals covering the complete data confidence interval for each method for the HTE estimand (interaction effect estimand $\gamma_3$)

| **Scenario** | **CCA** | **SI** | **MI** | **MMI** | **B-MMI** |
|---|---|---|---|---|---|
| Scenario 1 | 0.356 | 0.144 | 0.598 | 0.618 | 0.666 |
| Scenario 2 | 0.340 | 0.194 | 0.606 | 0.632 | 0.694 |
| Scenario 3 | 0.316 | 0.206 | 0.574 | 0.610 | 0.692 |
